# Supplementary material for: Stable Boundary Conditions and Discretization for PN Equations
Source: arXiv:2004.02497 source file (2021-01-18)
Supplement: Supplementary file 1 [file appendix.tex]

\appendix

\def\ustaggered{
	\begin{pmatrix}
		u^{ooo}\\ u^{ooe}\\ u^{oeo}\\ u^{oee}\\ 
		u^{eoo}\\ u^{eoe}\\ u^{eeo}\\ u^{eee}
\end{pmatrix}}
\def\Axstaggered{
	\begin{pmatrix}
		0 & 0 & 0 & 0 & A_1^{ooo} & 0 & 0 & 0 \\
		0 & 0 & 0 & 0 & 0 & A_1^{ooe} & 0 & 0 \\
		0 & 0 & 0 & 0 & 0 & 0 & A_1^{oeo} & 0 \\
		0 & 0 & 0 & 0 & 0 & 0 & 0 & A_1^{oee} \\
		A_1^{eoo} & 0 & 0 & 0 & 0 & 0 & 0 & 0 \\
		0 & A_1^{eoe} & 0 & 0 & 0 & 0 & 0 & 0\\
		0 & 0 & A_1^{eeo} & 0 & 0 & 0 & 0 & 0\\
		0 & 0 & 0 & A_1^{eee} & 0 & 0 & 0 & 0\\
\end{pmatrix}}
\def\Aystaggered{
	\begin{pmatrix}
		0 & 0 & A_2^{ooo} & 0 & 0 & 0 & 0 & 0 \\
		0 & 0 & 0 & A_2^{ooe} & 0 & 0 & 0 & 0 \\
		A_2^{oeo} & 0 & 0 & 0 & 0 & 0 & 0 & 0 \\
		0 & A_2^{oee} & 0 & 0 & 0 & 0 & 0 & 0 \\
		0 & 0 & 0 & 0 & 0 & 0 & A_2^{eoo} & 0 \\
		0 & 0 & 0 & 0 & 0 & 0 & 0 & A_2^{eoe}\\
		0 & 0 & 0 & 0 & A_2^{eeo} & 0 & 0 & 0\\
		0 & 0 & 0 & 0 & 0 & A_2^{eee} & 0 & 0\\
\end{pmatrix}}
\def\Azstaggered{
	\begin{pmatrix}
		0 & A_3^{ooo} & 0 & 0 & 0 & 0 & 0 & 0 \\
		A_3^{ooe} & 0 & 0 & 0 & 0 & 0 & 0 & 0 \\
		0 & 0 & 0 & A_3^{oeo} & 0 & 0 & 0 & 0 \\
		0 & 0 & A_3^{oee} & 0 & 0 & 0 & 0 & 0 \\
		0 & 0 & 0 & 0 & 0 & A_3^{eoo} & 0 & 0 \\
		0 & 0 & 0 & 0 & A_3^{eoe} & 0 & 0 & 0\\
		0 & 0 & 0 & 0 & 0 & 0 & 0 & A_3^{eeo}\\
		0 & 0 & 0 & 0 & 0 & 0 & A_3^{eee} & 0\\
\end{pmatrix}}
\begin{align}
\partial_t \ustaggered 
= &\Axstaggered \partial_{x_{1}} \ustaggered\\
+ &\Aystaggered \partial_{x_{2}} \ustaggered\\
+ &\Azstaggered \partial_{x_{3}} \ustaggered	
\label{appendix:PNequationStructure}
\end{align}

\begin{align}
&\frac{1}{2} \partial_t \sum_{\star\in M^3} \langle u^{\star}_h, u^\star_h \rangle_{\star}\\
&= \sum_{\star\in M^3} \langle u^{\star}_h, \partial_t u^\star_h \rangle_{\star}\\
&= \sum_{\star\in M^3} \langle u^{\star}_h, \sum_{i=1}^3 \mathcal{D}_i^\star (A_i^\star u^{c_i(\star)}) \rangle_{\star}\\
&= \sum_{\star\in M^3} \langle u^{\star}_h, 
\mathcal{P}^\star \mathcal{D}_1^\star (A_1^\star u_h^{c_1(\star)}) + 
\mathcal{P}^\star \mathcal{D}_2^\star (A_1^\star u_h^{c_2(\star)}) + 
\mathcal{P}^\star \mathcal{D}_3^\star (A_1^\star u_h^{c_3(\star)}) \rangle\\
&= \sum_{\star\in M^3} \langle u^{\star}_h, 
(\mathcal{Q}_x^{\star_1} \otimes \mathcal{P}_y^{\star_2} \otimes \mathcal{P}_z^{\star_3}) (A_1^\star u_h^{c_1(\star)}) + 
(\mathcal{P}_x^{\star_1} \otimes \mathcal{Q}_y^{\star_2} \otimes \mathcal{P}_z^{\star_3}) (A_1^\star u_h^{c_2(\star)}) + 
(\mathcal{P}_x^{\star_1} \otimes \mathcal{P}_y^{\star_2} \otimes \mathcal{Q}_z^{\star_3}) (A_1^\star u_h^{c_3(\star)}) \rangle\\
&= \sum_{\star\in M^2} \langle u^{o\star_1\star_2}_h, 
(\mathcal{Q}_x^{o} \otimes \mathcal{P}_y^{\star_1} \otimes \mathcal{P}_z^{\star_2}) (A_1^{o\star_1\star_2} u_h^{{e\star_1\star_2}}) \rangle +
\langle u^{e\star_1\star_2}_h, 
(\mathcal{Q}_x^{e} \otimes \mathcal{P}_y^{\star_1} \otimes \mathcal{P}_z^{\star_2}) (A_1^{e\star_1\star_2} u_h^{{o\star_1\star_2}}) \rangle \\
&\qquad+ \langle u^{\star_1 o \star_2}_h, 
(\mathcal{P}_x^{\star_1} \otimes \mathcal{Q}_y^{o} \otimes \mathcal{P}_z^{\star_2}) (A_1^{\star_1 o\star_2} u_h^{{\star_1 e\star_2}}) \rangle +
\langle u^{\star_1 e\star_2}_h, 
(\mathcal{P}_x^{\star_1} \otimes \mathcal{Q}_y^{e} \otimes \mathcal{P}_z^{\star_2}) (A_1^{\star_1 e\star_2} u_h^{{\star_1 o\star_2}}) \rangle \\
&\qquad+ \langle u^{\star_1\star_2 o}_h, 
(\mathcal{P}_x^{\star_1} \otimes \mathcal{P}_y^{\star_2} \otimes \mathcal{Q}_z^{o}) (A_1^{\star_1\star_2 e} u_h^{{\star_1\star_2 e}}) \rangle +
\langle u^{\star_1\star_2 e}_h, 
(\mathcal{P}_x^{\star_1} \otimes \mathcal{P}_y^{\star_2} \otimes \mathcal{Q}_z^{e}) (A_1^{\star_1\star_2 e} u_h^{{\star_1\star_2 o}}) \rangle \\
&= \sum_{\star\in M^2} \langle u^{o\star_1\star_2}_h, 
(\mathcal{Q}_x^{o} \otimes \mathcal{P}_y^{\star_1} \otimes \mathcal{P}_z^{\star_2}) (A_1^{o\star_1\star_2} u_h^{{e\star_1\star_2}}) \rangle +
\langle u^{o\star_1\star_2}_h, 
({\mathcal{Q}_x^{e}}^{T} \otimes \mathcal{P}_y^{\star_1} \otimes \mathcal{P}_z^{\star_2}) (A_1^{o\star_1\star_2} u_h^{{e\star_1\star_2}}) \rangle \\
&\qquad+ \langle u^{\star_1 o \star_2}_h, 
(\mathcal{P}_x^{\star_1} \otimes \mathcal{Q}_y^{o} \otimes \mathcal{P}_z^{\star_2}) (A_1^{\star_1 o\star_2} u_h^{{\star_1 e\star_2}}) \rangle +
\langle u^{\star_1 o \star_2}_h, 
(\mathcal{P}_x^{\star_1} \otimes {\mathcal{Q}_y^{e}}^T \otimes \mathcal{P}_z^{\star_2}) (A_1^{\star_1 o\star_2} u_h^{{\star_1 e\star_2}}) \rangle \\
&\qquad+ \langle u^{\star_1\star_2 o}_h, 
(\mathcal{P}_x^{\star_1} \otimes \mathcal{P}_y^{\star_2} \otimes \mathcal{Q}_z^{o}) (A_1^{\star_1\star_2 e} u_h^{{\star_1\star_2 e}}) \rangle +
\langle u^{\star_1\star_2 e}_h, 
(\mathcal{P}_x^{\star_1} \otimes \mathcal{P}_y^{\star_2} \otimes {\mathcal{Q}_z^{e}}^T) (A_1^{\star_1\star_2 o} u_h^{{\star_1\star_2 e}}) \rangle \\
&= \sum_{\star\in M^2} \langle u^{o\star_1\star_2}_h, 
((\mathcal{Q}_x^{o}+{\mathcal{Q}_x^{e}}^{T}) \otimes \mathcal{P}_y^{\star_1} \otimes \mathcal{P}_z^{\star_2}) (A_1^{o\star_1\star_2} u_h^{{e\star_1\star_2}}) \rangle \\
&\qquad+ \langle u^{\star_1 o \star_2}_h, 
(\mathcal{P}_x^{\star_1} \otimes (\mathcal{Q}_y^{o}+ {\mathcal{Q}_y^{e}}^T) \otimes \mathcal{P}_z^{\star_2}) (A_1^{\star_1 o\star_2} u_h^{{\star_1 e\star_2}}) \rangle \\
&\qquad+ \langle u^{\star_1\star_2 o}_h, 
(\mathcal{P}_x^{\star_1} \otimes \mathcal{P}_y^{\star_2} \otimes (\mathcal{Q}_z^{o}+{\mathcal{Q}_z^{e}}^T)) (A_1^{\star_1\star_2 e} u_h^{{\star_1\star_2 e}}) \rangle \\
&= \sum_{\star\in M^2} \langle u^{o\star_1\star_2}_h, 
(\mathcal{B}_x \otimes \mathcal{P}_y^{\star_1} \otimes \mathcal{P}_z^{\star_2}) (A_1^{o\star_1\star_2} u_h^{{e\star_1\star_2}}) \rangle \\
&\qquad+ \langle u^{\star_1 o \star_2}_h, 
(\mathcal{P}_x^{\star_1} \otimes \mathcal{B}_y \otimes \mathcal{P}_z^{\star_2}) (A_1^{\star_1 o\star_2} u_h^{{\star_1 e\star_2}}) \rangle + \langle u^{\star_1\star_2 o}_h, 
(\mathcal{P}_x^{\star_1} \otimes \mathcal{P}_y^{\star_2} \otimes \mathcal{B}_z) (A_1^{\star_1\star_2 o} u_h^{{\star_1\star_2 e}}) \rangle \\
\end{align}
